# Supplementary material for: Natural Language Supervision for General-Purpose Audio Representations
Source: arXiv:2309.05767 source file (2024-02-06)
Supplement: Supplementary file 1 [file appendix.tex]

\section{Training datasets} \label{appendix: training datasets}

\noindent \textbf{FSD50k}~\cite{fsd50k} is a sound event classification dataset with audio clips from freesound.org. The duration of the clips ranges from 0.3 to 30 seconds. We used the ~36k clips from training and validation. We constructed the caption for each clip by concatenating the two sentences the associated title and description in the metadata. We ignored the class label. \\
\textbf{ClothoV2} \cite{clotho} is an audio captioning dataset consisting of ~7k audio clips. The duration of the clips range from 15 to 30 seconds. Each clip has 5 captions annotated by different participants. Thus, we created 5 pairs for each clip extending the number of audio-text pairs by 5 times. \\
\textbf{AudioCaps} \cite{audiocaps} is an audio captioning dataset consisting of ~46k audio clips from AudioSet. The duration of the clips is 10 seconds. Each clip has a caption annotated via crowd-sourcing. \\
\textbf{MACS} \cite{macs} is an audio captioning dataset consisting of ~4k audio clips. The duration of the clips is 10 seconds. Each clip is captioned by multiple participants. Similar to ClohtoV2, we paired the same audio with a each of their associated captions to create a larger set of pairs consisting of ~17k. 
At the time of downloading the datasets, not all clips were available from the web links.

\begin{table}[ht]
\center
\begin{tabular}{lccc} \hline
Dataset & Pairs & \makecell{Unique\\ audios} & \makecell{Unique \\captions} \\ \hline
FSD50k & 36,796 & 36,796 & 36,796 \\
ClothoV2 & 29,646 & 5,929 & 29,646 \\
AudioCaps & 44,292 & 44,292 & 44,292 \\
MACS & 17,276 & 3,930 & 17,276 \\ \hline
 & 128,010 & 90,947 & 128,010 \\ \hline
\end{tabular}
\caption{\label{table: training dataset}
Training dataset statistics. \vspace{-0.08in}}
\end{table}

\begin{table*}[ht]
\small
\center
\begin{tabular}{ccccccccc}\hline
 Domain & Dataset & Files & Dur. (secs) & Classes & Metric & Setup \\ \hline
\multirowcell{5}{
 Sound Event  \\ Classification (SEC)} & ESC50 & 2k & 5 & 50 & ACC & 5 folds \\
 & FSD50K & ~51k & 0.3 - 30 & 200 & mAP & train/val/test \\
 & UrbanSound8K & ~8k & $\leq$ 4 & 10 & ACC & 10 folds \\
 & DCASE2017 Task4 & 52k & 10 & 17 & ACC & train/val/test \\
 & AudioSet & $\sim$2M & 10 & 527 & mAP & train/val/test \\ \hline
% Acoustic \\ Scenes & Some dataset &  &  &  & ? &  \\ \hline
\multirowcell{5}{Music} & GTZAN Music Speech & 120 & 30 & 2 & ACC & 10 folds \\
 & GTZAN Music Genre & 1k & 30 & 10 & ACC & 10 folds \\
 & Mridangam Stroke & ~7k & 0.81 & 10 & ACC & 5 folds \\
 & Mridangam Tonic & ~7k & 0.81 & 6 & ACC & 5 folds \\ \hline
\makecell{Instrument \\ Classification} & \makecell{Beijing Opera \\ Percussions} & 236 & 4.77 & 4 & ACC & 5 folds \\ \hline
\makecell{Acoustic Scene \\ Classification} & TUT 2017 & 6.3k & 10 & 15 & ACC & train/val/test \\ \hline
\multirowcell{2}{Emotion \\ Recognition} & CREMA-D & ~7k & 5 & 6 & ACC & 5 folds \\
 & RAVDESS & ~2.5k & $\leq$ 5 & 8 & ACC & 5 folds \\ \hline
% Bio \\ Acoustics & Beehive states & 930 & 600 & 2 & ACC & train/val/test \\ \hline
Keyword \\ Spotting & Speech Commands & 100k & 1 & 12 & ACC & train/val/test \\ \hline
\makecell{Vocal Sound \\ Classification} & \makecell{Vocal Sound} & ~21k & 5 & 6 & ACC & train/val/test \\ \hline
Speaker Counting & LibriCount 10 & 5k & 5 &  11 & ACC & 5 folds \\\hline
\end{tabular}
\caption{\label{table: downstream datasets}
Details from the 16 datasets used as Downstream Tasks.
}
\end{table*}

\section{Downstream datasets} \label{appendix: downstream datasets}
\vspace{-0.05in}
\textbf{ESC50} is an environmental classification dataset comprising of 50 events. The dataset consists of 2k files of 5 seconds each. The evaluation setup is 5 fold cross validation and the evaluation metric is accuracy. \\
\textbf{FSD50K} is a sound event classification dataset comprising of 200 events. The dataset consists of 51k files ranging from 0.3 to 30 seconds each. The evaluation setup is train/val/test and the evaluation metric is mAP. \\
\textbf{UrbanSound8K} is urban sound classification dataset comprising of 10 sounds. The dataset consists of 8k files of ~4 seconds each. The evaluation setup is 10 fold cross validation and the evaluation metric is accuracy. \\
\textbf{DCASE2017 Task4} is a sound event classification dataset comprising of 17 sounds recorded in domestic environment. The dataset consists of ~30k files of 10 seconds each. The evaluation setup is train/val/test and the evaluation metric is accuracy. \\
\textbf{AudioSet} is a sound event classification dataset comprising of 527 sounds from YouTube videos. The dataset consists of ~2M files of 10 seconds each. The evaluation setup is train/val/test and the evaluation metric is accuracy. \\
\textbf{TUT 2017} is an acoustic scene classification dataset comprising of 15 acoustic scenes in both outdoor and indoor environment. The dataset consists of ~52k files of 10 seconds each. The evaluation setup is train/val/test and the evaluation metric is accuracy.\\ 
\textbf{GTZAN Music Speech} is a binary classification dataset where the aim is to distinguish between human speech and music. The dataset consists of 120 files of 30 seconds each. The evaluation setup is 10 fold cross validation and the evaluation metric is accuracy. \\
\textbf{GTZAN Genres} is music genre classification dataset comprising of 10 genres. The dataset consists of 1k files of 30 seconds each. The evaluation setup is 10 fold cross validation and the evaluation metric is accuracy. \\
\textbf{Mridangam Stroke} is music stroke classification dataset comprising of 10 strokes from Mridangam (pitched percussion instrument). The dataset consists of 1k files of 0.81 seconds each. The evaluation setup is 5 fold cross validation and the evaluation metric is accuracy. \\
\textbf{Mridangam Tonic} is music tonic classification dataset comprising of 6 tonics from Mridangam (pitched percussion instrument). The dataset consists of 1k files of 0.81 seconds each. The evaluation setup is 5 fold cross validation and the evaluation metric is accuracy. \\
\textbf{Beijing Opera Percussions} is an instrument classification dataset comprising of 4 percussion instruments from Beijing Opera. The dataset consists of 236 files of 4.77 seconds each. The evaluation setup is 5 fold cross validation and the evaluation metric is accuracy. \\
\textbf{CREMA-D} is an emotion recognition dataset comprising of 6 emotions. The dataset consists of ~7k files of 5 seconds each. The evaluation setup is 5 fold cross validation and the evaluation metric is accuracy. \\
\textbf{RAVDESS} is an emotion recognition dataset comprising of 8 emotions. The dataset consists of ~2.5k files of 5 seconds each. The evaluation setup is 5 fold cross validation and the evaluation metric is accuracy. \\
\textbf{Speech Commands V2} is an keyword spotting dataset comprising of 13 commands. The dataset consists of 100k files of 1 seconds each. The evaluation setup is train/val/test and the evaluation metric is accuracy.\\
\textbf{Vocal Sound} is a human vocal sound classification dataset comprising of 6 vocalizations. The dataset consists of 21k files of 5 seconds each. The evaluation setup is train/val/test and the evaluation metric is accuracy.\\
\textbf{LibriCount} is a speaker count estimation dataset comprising of simulated cocktail party environment audios consisting of 0 to 10 speakers. The dataset consists of 5k files of 5 seconds each. The evaluation setup is 5 fold cross validation and the evaluation metric is accuracy. \\
